# Supplementary material for: A first look into the carbon footprint of federated learning
Source: arXiv:2102.07627 source file (2023-05-22)
Supplement: Supplementary file 1 [file 6_appendix.tex]

\appendix
\section{Appendix}
\label{sec:appendix}

\subsection{Detailed results on CIFAR10 and ImageNet experiments}
\label{ap:timeresults}

This section enriches the results described in section \ref{sec:estimation} with training times and number of rounds needed to compute the reported CO$_2$e estimate. All the results are given in Table \ref{tab:cifartime}.

\begin{table}[!h]
\centering
\scalebox{0.8}{
\begin{tabular}{p{3.2cm}|P{1.5cm}|P{1.5cm}P{1.5cm}|P{1.25cm}|P{2.25cm}}
\toprule
\textbf{Setup} & \textbf{Hardware} & \multicolumn{2}{ |c| }{\textbf{Rounds or Epochs}} & \textbf{Time (s)} & \textbf{Max Acc. (\%)}\\ 
\textbf{CIFAR10}&&$50 \%$&$60 \%$&& \\
\midrule
centralized Training & V100 & 1 & 2 & 48 & $71.0$ \\
centralized Training & K80 & 1 &2& 84 & $71.0$ \\
FL (IID, 1 epoch) & Tegra X2 & 5 & 16 & 51.4 & $64.3$ \\
FL (IID, 5 epoch) & Tegra X2 & 4 & 9 & 257 & $65.0$ \\
FL (non-IID, 1 epoch) & Tegra X2 & 20 & 75 & 51.4 & $61.0$ \\
FL (non-IID, 5 epoch) & Tegra X2 & 5 & 11 & 257 & $63.5$ \\
\bottomrule
\end{tabular}
}
\vspace*{0.3cm}

\scalebox{0.8}{

\begin{tabular}{p{3.5cm}|p{2cm}|p{3cm}|p{1.5cm}}
\toprule
\textbf{Setup} & \textbf{Hardware} & \textbf{Rounds or Epochs} & \textbf{Time (s)} \\ 
\textbf{ImageNet}& &$50 \%$& \\
\midrule
centralized Training & V100 & 5  & 3,840  \\
FL (IID, 3 epochs) & Tegra X2 & 25 & 3,840 \\
\bottomrule
\end{tabular}
}
\captionsetup{font=small,labelfont=bf}
\caption{ Run time results for FL and centralized training on the CIFAR10 (top table) and ImageNet (bottom table) datasets. “IID” and “non-IID” terms are employed to distinguish between clients that have an evenly distributed set of samples containing all the classes (IID) and clients that have more samples of certain classes (non-IID). The ``Time'' column corresponds to the run time per epoch for centralized training or run time per communication round for FL. The ``Max Acc.'' column reports the maximum testing accuracy obtained. Finally, the ``Rounds or Epochs'' column gives the number of rounds or epochs needed to reach the indicated level of testing accuracy.}
\label{tab:cifartime}
\end{table}

It is worth noting that in this setup, FL is slower and offers worst performance compared to centralized training on CIFAR10. Since each client has $1/10$ of the total dataset, each \textit{local} epoch can be seen as $1/10$ of a \textit{global} epoch. The accuracy difference could be explained by the simple FedAVG strategy employed for FL that could lead to a loss of information through the weight averaging performed at each communication round, or by a shift in the running statistics contained in the batch-normalisation layers of the ResNet-18 model. Indeed, FedAVG averages the latter statistics certainly leading to a small shift at every round. However, better performance may also be obtained with FL as shown in Figure \ref{fig:carbonefficiency} by simply considering better setups (\textit{i.e} number of clients, number of local epochs ...).

\textbf{Carbon emission estimation example.}  Eq. \ref{eq:carboneq} can be applied to Table \ref{tab:cifartime} to compute the CO$_2$e emitted to reach $50$\% of accuracy with the \textit{FL (IID, 5 epoch)}  setup as:
\begin{align}
   16\times0.9746\times5\times(\frac{51.4}{3600}\times10)=11.13g,
\end{align}

with $16$ the number of rounds, $0.9746$ the energy conversion rate of China, $5$ the number of selected clients, $51.4$ the time in seconds needed to complete one round and $10$ the power by the Nvidia TX2. 

\subsection{Carbon footprint estimation with FashionMNIST}
\label{ap:fashion}
The CO$_2$e estimation methodology detailed in section \ref{sec:datacentre} and applied to CIFAR10 and ImageNet in section \ref{sec:estimation} is extended in this section to the FashionMNIST dataset for further context. 

FashionMNIST consists in $60,000$ training images of size $28\times28$ distributed across $10$ classes, and $10,000$ test samples. Since there is no natural user partitioning of this dataset, we follow the same IID and non-IID protocol than for the CIFAR10 experiments. However, for the sake of diversity, the model architecture considered for this experiment is reduced to a simple CNN with two convolutional layers with a kernel size of $5$, followed with $2$ fully connected layer composed by $512$ hidden neurons and a final layer of size $10$. In this setup, each client only performs $1$ local epoch per round. 

\begin{table}[!t]
\centering
\scalebox{0.8}{
\begin{tabular}{p{3.2cm}|P{1.5cm}|P{1.5cm}P{1.5cm}|P{1.25cm}|P{2.25cm}}
\toprule
\textbf{Setup} & \textbf{Hardware} & \multicolumn{2}{ |l| }{\textbf{Rounds or Epochs}} & \textbf{Time (s)} & \textbf{Max Acc. (\%)}\\ 
\textbf{FashionMNIST}&&$85 \%$&$90 \%$&& \\
\midrule
centralized Training & V100 & 2 & 5 & 5 & $92.0$ \\
centralized Training & K80 & 2 &5 & 13.5 &  $92.0$ \\
FL (IID, 1 epoch) & Tegra X2 & 8 & 26 & 5.6 & $92.0$ \\
FL (non-IID, 1 epoch) & Tegra X2 & 30 & 50 & 5.6 & $91.0$ \\
\bottomrule
\end{tabular}
}
\captionsetup{font=small,labelfont=bf}
\caption{Run time results for FL and centralized training on the FashionMNIST dataset. “IID” and “non-IID” terms are employed to distinguish between clients that have an evenly distributed set of samples containing all the classes (IID) and clients that have more samples of certain classes (non-IID). The ``Time'' column corresponds to the run time per epoch for centralized training or run time per communication round for FL. The ``Max Acc.'' column reports the maximum testing accuracy obtained. Finally, the ``Rounds or Epochs'' column gives the number of rounds or epochs needed to reach the indicated level of testing accuracy.}
\label{tab:mnistresult}
\end{table}

Table \ref{tab:mnistresult} reports the run time observed with the different setups. As expected, FL remains slower compared to centralized training. However, due to the simplicity of the task and the neural network architecture, both FL and centralized learning achieve the same level of maximum accuracy ($92$\%). 

\begin{table}[t!]
\centering
\scalebox{0.8}{
\begin{tabular}{p{2.4cm}|P{0.75cm}P{0.75cm}|P{0.75cm}P{0.75cm}|P{1.2cm}P{1.25cm}| P{1.2cm}P{1.25cm} }
\toprule
 \textbf{Country/CO2(g)}& \textbf{V100} & \textbf{K80} &\textbf{V100} & \textbf{K80} & \textbf{FL} & \textbf{FL}\\ 

& \multicolumn{2}{ |c| }{$PUE = 1.67$} & \multicolumn{2}{ |c| }{$PUE = 1.11$} & IID &non-IID \\
% &$PUE = 1.67$ & & $PUE = 1.11$ &  &\\
\midrule
 USA &1.6 & 5.2  &1.1& 3.5& 1.1 & 2.1 \\
 China &2.9 & 9.2 &1.9 & 6.2 & 2.0 & 3.8\\
 France & 0.2 & 0.8 & 0.2 & 0.5 & 0.2 & 0.3\\
\bottomrule
\end{tabular}
}
\captionsetup{font=small,labelfont=bf}
\caption{CO$_2$e emissions (expressed in grams, i.e \textbf{lower is better}) for centralized training and FL on FashionMNIST. Emissions are calculated once the top-1 accuracy on the test set reaches $90$\%. The number of epoch reported on the FL column relates to the number of local epoch done per client. ``IID'' and ``non-IID'' terms are employed to distinguish between clients that have an evenly distributed set of samples containing all the classes (IID) and clients that have more samples of certain classes (non-IID).}
\label{tab:mnist}
\end{table}

Interestingly, with such a simple task, FL is almost as efficient as centralized training while considering Tesla V100. Hence, FL is even greener than a datacenter solution relying on Tesla K80. In summary, and has already shown in section \ref{sec:estimation}, the comparison between FL and centralized training highly depends on: 1. the efficiency of the considered datacenter (\textit{i.e.} PUE and GPU efficiency). 2. The partitioning of the FL dataset (\textit{i.e.} IID vs non-IID). 3. The FL setup.

\subsection{Detailed optimization results}
\label{ap:opti}

The necessary details to produce Figure \ref{fig:carbonefficiency} and Figure \ref{fig:resultsgrowth} are reported in this Appendix. All models are trained on the CIFAR10 dataset. The number of randomly selected clients vary from $1$ to $10$ and the number of local epochs is either $1$ or $5$. We also propose to consider IID and non-IID partitioning as this setup has been shown to strongly impact the final results. 

Table \ref{tab:allopti} shows that FL remains carbon efficient until the fine-tuning phase is reached. As an example, reaching $60$\% of accuracy on the test set with $5$ local epochs and an IID partitioning emits $5.47$g of CO$_2$e. Pushing this model to $68.6$\% of accuracy increases the amount of carbon to $97.64$g. Such a phenomenon is easily explained by the larger number of round needed to properly fine-tune the model (\textit{i.e.} also true with centralized training). However, it also shows that a trade off between CO$_2$e and precision could be found. Finally, and as depicted with other experiments, a non-IID partitioning of the data (\textit{i.e.} more realistic) causes a important increase of the pollution.

\begin{table}[h!]
\centering
\scalebox{0.8}{
\begin{tabular}{P{3.5cm}|P{1cm}P{1.5cm}P{2cm}|P{1cm}P{1cm}P{1.5cm}P{2cm}}
\toprule

\textbf{Clients/round} &  \multicolumn{3}{ |c| }{\textbf{ Test Acc $60 \%$} }&  \multicolumn{4}{ |c }{\textbf{Stable Acc} } \\ 
\textbf{IID, 5 local epochs}& \textbf{Rounds} & \textbf{CO$_{2}$ (g)} & \textbf{Carbon Cost} & \textbf{Acc} & \textbf{Rounds} & \textbf{CO$_{2}$ (g)} &\textbf{Carbon Cost}\\

\midrule
1 & 14 & 5.47 & \textbf{9.11} & $68.6 \%$ & 250 & 97.64 & 142.33 \\
2 & 14 & 10.94 & 18.23 & $66.0 \%$  & 82   & 64.05   & 97.05\\
3 & 9 & 10.55 & 17.58 & $65.3 \%$  & 50   & 58.58  & 89.72 \\
4 & 9 & 14.06 & 23.43 & $66.0 \%$  & 40  & 62.49   & 94.68 \\
5 & 9 & 17.58 & 29.29 & $65.0 \%$  & 35   & 68.35  & 105.15 \\
6 & 8 & 18.75 & 31.25  & $64.5 \%$  & 18  & 42.18  & 65.40\\
7 & 8 & 21.87  & 36.45  & $64.5 \%$  & 15  & 41.01  & \textbf{63.58}\\
8 & 7 & 21.87 & 36.45 & $64.5 \%$  & 16  & 49.99  &  77.51 \\
9 & 8 & 28.12 & 46.87  & $64.5 \%$  & 16  & 56.24  & 87.20 \\
10 & 8 & 31.25 & 52.08  & $64.5 \%$  & 16  & 70.30  & 109.00 \\

\bottomrule
\end{tabular}
}

\centering
\scalebox{0.8}{
\begin{tabular}{P{3.5cm}|P{1cm}P{1.5cm}P{2cm}|P{1cm}P{1cm}P{1.5cm}P{2cm}}
\toprule

\textbf{Clients/round} &  \multicolumn{3}{ |c| }{\textbf{ Test Acc $60 \%$} }&  \multicolumn{4}{ |c }{\textbf{Stable Acc} } \\ 
\textbf{IID, 1 local epochs}& \textbf{Rounds} & \textbf{CO$_{2}$ (g)} & \textbf{Carbon Cost} & \textbf{Acc} & \textbf{Rounds} & \textbf{CO$_{2}$ (g)} &\textbf{Carbon Cost}\\

\midrule
1 & 28  & 2.19 & \textbf{3.65} & $70.2 \%$ & 330 & 25.78 & 36.72 \\
2 & 24 & 3.75 & 6.25 & $67.0 \%$ &  200 & 31.25 & 46.63\\
3 & 19 & 4.45 & 7.42 & $66.2 \%$ & 100 & 23.43 & 35.40\\
4 & 16 & 5.00 & 8.33 & $64.0 \%$ & 70 & 21.87 &\textbf{34.17}\\
5 & 16 & 6.25 & 10.42 & $64.3 \%$ & 73 & 28.51 & 44.34\\
6 & 16 & 7.50 & 12.50 & $63.7\%$ & 68 & 31.87 & 50.03\\
7 & 17 & 9.30 & 15.49 & $62.7 \%$ & 61 & 33.35 & 53.20\\
8 & 16 & 10.00 & 16.66 & $63.0 \%$ & 55 & 34.37 & 54.56\\
9 & 14 & 9.84 & 16.40 & $63.0 \%$ & 40 & 28.12 & 44.64\\
10 & 17 & 13.28  & 22.13 &  $62.5 \%$ & 45 &  35.15 & 56.24\\

\bottomrule
\end{tabular}
}

\scalebox{0.8}{
\begin{tabular}{P{3.5cm}|P{1cm}P{1.5cm}P{2cm}|P{1cm}P{1cm}P{1.5cm}P{2cm}}
\toprule

\textbf{Clients/round} &  \multicolumn{3}{ |c| }{\textbf{ Test Acc $60 \%$} }&  \multicolumn{4}{ |c }{\textbf{Stable Acc} } \\ 
\textbf{non-IID, 5 local epochs}& \textbf{Rounds} & \textbf{CO$_{2}$ (g)} & \textbf{Carbon Cost} & \textbf{Acc} & \textbf{Rounds} & \textbf{CO$_{2}$ (g)} &\textbf{Carbon Cost}\\

\midrule
1 & 43 & 16.79 & 27.99 & $65.5 \%$ & 250 & 97.64 & 149.07 \\
2 & 16 & 12.50 & \textbf{20.83} & $65.3 \%$ & 190 & 148.41 & 227.28 \\
3 & 15 & 17.58 & 29.29 & $64.7 \%$ & 90 & 105.45 & 162.99 \\
4 & 12 & 18.75 & 31.25 & $63.7 \%$ & 50 & 78.11 & 122.63 \\
5 & 11 & 21.48 & 35.80 & $63.5 \%$ & 40 & 78.11 & 123.01 \\
6 & 12 & 28.12 & 46.87 & $63.5 \%$ & 40 & 93.74 & 147.62 \\
7 & 10 & 27.34 & 45.57 & $63.5 \%$ & 40 & 109.36 & 172.22\\
8 & 11 & 34.37 & 57.28 & $62.0 \%$ & 19 & 59.37 & 95.75 \\
9 & 10 & 35.15 & 58.58 & $62.0 \%$ & 17 & 59.76 & 96.38 \\
10 & 9 & 35.15 & 58.58 & $62.3 \%$ & 14 & 54.68 & \textbf{87.77} \\

\bottomrule
\end{tabular}
}

\scalebox{0.8}{
\begin{tabular}{P{3.5cm}|P{1cm}P{1.5cm}P{2cm}|P{1cm}P{1cm}P{1.5cm}P{2cm}}
\toprule

\textbf{Clients/round} &  \multicolumn{3}{ |c| }{\textbf{ Test Acc $60 \%$} }&  \multicolumn{4}{ |c }{\textbf{Stable Acc} } \\ 
\textbf{non-IID, 1 local epochs}& \textbf{Rounds} & \textbf{CO$_{2}$ (g)} & \textbf{Carbon Cost} & \textbf{Acc} & \textbf{Rounds} & \textbf{CO$_{2}$ (g)} &\textbf{Carbon Cost}\\

\midrule
1 & 250 & 19.53 & \textbf{32.55} & $66.8 \%$  & 450  & 35.15 & \textbf{52.62}\\
2 & 135 & 21.09 & 35.15 & $64.5 \%$ & 330  & 51.55 & 79.93 \\
3 & 90  & 21.09 & 35.15 & $62.8 \%$ & 300  & 70.30 & 111.95\\
4 & 75 & 23.43 & 39.06 & $62.8 \%$ & 160  & 49.99 & 79.61\\
5 & 75 & 29.29 & 48.82 & $61.0 \%$ & 140  & 54.68 & 89.64\\
6 & 75 & 35.15 & 58.58 & $61.5 \%$ & 130  & 60.93 & 99.07\\
7 & 60  & 32.81 & 54.68 & $60.0 \%$ & 60  & 32.81 & 54.68\\
8 & NA & NA & NA & $59.0\%$ & 60  & 37.49 & 63.55\\
9 & NA  & NA & NA & $58.0 \%$ & 50  & 35.15 & 60.61\\
10 & NA & NA & NA  & $58.8 \%$ &  60  & 46.87 & 79.70\\

\bottomrule

\end{tabular}
}
\captionsetup{font=small,labelfont=bf}
\caption{ Details of the results obtained on CIFAR10 with multiple FL setups. “IID” and “non-IID” terms are employed to distinguish between clients that have an evenly distributed set of samples containing all the classes (IID) and clients that have more samples of certain classes (non-IID). The ``Max Acc.'' column reports the maximum testing accuracy obtained. The ``Rounds'' column gives the number of rounds needed to reach the indicated level of testing accuracy. Finally, ``Carbon Cost'' numbers are obtained by applying Eq. \ref{eq:carboncost} (lower is better).}
\centering
\label{tab:allopti}
\end{table}
